# Supplementary material for: Local free energy approximations for the coarse-graining of adsorption phenomena
Source: arXiv:1801.06158 source file (2018-01-18)
Supplement: Supplementary file 1 [file Pazzona_jan_2018_SuppInfo.pdf]

# Local free energy approximations for the coarse-graining of adsorption phenomena

Federico G. Pazzona,\* Giovanni Pireddu, Andrea Gabrieli, Alberto Pintus, and Pierfranco Demontis  
*Dipartimento di Chimica e Farmacia, Università degli Studi di Sassari, via Vienna 2, 07100 Sassari, Italy*

As Supplementary Material, we provide (1) single-cell and cell-pair probability distributions for the occupancy of the lattice-gas system investigated in the main article, (2) lone-pore-pair isotherms and related coarse-grained results under the non-interacting pair approximation for the Lennard-Jones system (united-atom methane in static ITQ-29 zeolite), and (3) single-pore and pore-pair probability distributions for the occupancy of the same Lennard-Jones system. We also describe and comment two strategies to estimate the coarse-grained interaction terms.

## I. OCCUPANCY DISTRIBUTIONS FOR THE LATTICE-GAS SYSTEM

We provide simulation data on the occupancy distributions of the lattice-gas system presented in the main article, where each cell can contain up to  $n_{\max} = 9$  particles. In each figure, the following probability distributions are shown for four selected fugacity values:  $p(n)$  (subfigure *a*), that indicates the probability for a single cell to host  $n$  particles, and  $p(n, m)$  (subfigures *b-e*), the joint probability of a pair of neighboring cells to have occupancies  $n, m$ . For each of the selected fugacities, the latter probability,  $p(n, m)$ , is shown in the form of four stacked plots, in every one of which  $n$  is kept fixed at a value close to the occupancy at which  $p(n)$  reaches its maximum. For example, in Fig. S1-*a* the maximum in the single-cell histogram  $p(\cdot)$  at fugacity  $f_1 = 2.49 \cdot 10^3$  bar (black color), is reached for occupancy  $n = 1$ ; the three most probable occupancies that are closest to  $n = 1$  are  $n = 0$ ,  $n = 2$ , and  $n = 3$ , therefore Fig. S1-*b* we show, beside the histogram of  $p(1, \cdot)$ , also the histograms of  $p(0, \cdot)$ ,  $p(2, \cdot)$ , and  $p(3, \cdot)$ . As the histogram of  $p(\cdot)$  was in black color, also the stacked histograms  $p(0, \cdot)$ ,  $p(1, \cdot)$ ,  $p(2, \cdot)$ , and  $p(3, \cdot)$  are drawn in black. Analogously, since the maximum of  $p(\cdot)$  at  $f_2 = 5.04 \cdot 10^4$  bar (red color) is reached at  $n = 3$ , and the other three most probable occupancies are  $n = 1$ ,  $n = 2$ , and  $n = 4$ , the stacked histograms in Fig. S1-*c* (also in red color) refer to  $p(1, \cdot)$ ,  $p(2, \cdot)$ ,  $p(3, \cdot)$ , and  $p(4, \cdot)$ . Obviously, the units for the stacked histograms are arbitrary (a.u.), with the lowest reported value of each histogram defining an invisible baseline of zero probability that applies only for that histogram. Both for the single-cell and the cell-pair probabilities, dots represent values estimated from the fine-grained (FG) simulation. Solid and dashed lines refer instead to the coarse-grained (CG) system, respectively simulated through the parameters obtained by the IPA and the NIPA approaches.

For every system we considered, the subfigure *f* reports the adsorption isotherm (reported also in the main article), i.e. the plot of the cell density, expressed as the average occupancy divided by the maximum occupancy,  $\langle n \rangle / n_{\max}$ , whereas in subfigure *g* we report the ‘extended density’, that we defined as the average of the product of the cell occupancy,  $n$ , times the sum of the occupancy in its whole neighborhood,  $M$ , divided by  $\nu n_{\max}$ ,  $\nu$  being the number of neighbors of each cell (for the lattice-gases we considered,  $\nu = 4$ ). The extended density,  $\langle nM \rangle / (\nu n_{\max})$ , gives us information on the correlation between the density in a single cell and the density in its whole neighborhood. We chosen to show it because, since the extended density was *not* matched directly in our coarse-graining, it is a property where FG and the CG system might, in principle, show some dissimilarities. In density and extended density plots, empty circles are used to represent data from the FG system, whereas solid black lines and dashed blue lines are used respectively for IPA and NIPA results.

In all the lattice-gas setups, the temperature was set to the indicative value of  $T = 200$  K.

In Fig. S1 we report data for the lattice-gas system in which the repulsion parameter is set to  $\epsilon = 5$  kJ mol<sup>-1</sup>, and in Fig. S2, we set the lateral repulsion to  $\epsilon = 8$  kJ mol<sup>-1</sup>. In such cases, the lattice-gas Hamiltonian is simply

$$E(\mathbf{s}) = \epsilon \sum_{\langle i, j \rangle} s_i s_j, \quad (\text{S1})$$

---

\*Electronic address: fpazzona@uniss.it

where the sum runs over all the pairs of neighboring sites, and  $s_i$  and  $s_j$  are the occupancies of sites  $i$  and  $j$  (each of them being either 0 if empty or 1 if occupied), according to the occupancy configuration  $\mathbf{s}$  of the whole FG lattice.

In Fig. S3 we set it back to  $\epsilon = 5 \text{ kJ mol}^{-1}$ , but we added a non-zero next-neighborhood attractive contribution (extended interactions) with parameters  $\phi = -1.6 \text{ kJ mol}^{-1}$  and  $M_0 = 4$ . In this case, the lattice-gas Hamiltonian is

$$E(\mathbf{s}) = \sum_{\langle i,j \rangle} s_i s_j \left[ \epsilon + \psi(M_i) + \psi(M_j) \right], \quad \psi(M) = \phi \sum_{m \geq M_0} \delta_{M,m}, \quad (\text{S2})$$

where  $M_i$  and  $M_j$  are defined as the total occupancy in the neighborhood, respectively, of site  $i$ , including the occupancy of  $j$ , and of site  $j$ , including the occupancy of  $i$  (see the main article for further details).

In all our lattice-gas simulations, the IPA approach provided a better match with the FG properties than the NIPA (nearly equal match at the lowest densities, where cell-cell correlations are relatively weak). In particular, the presence of extended interactions causes strong intercell correlations to emerge, in the original FG system (see Fig. S3). This is particularly evident at intermediate-high densities, i.e. in the nearness of the step in the adsorption isotherm. Under such conditions, the NIPA approach fails, whereas the IPA coarse-graining still holds. The case of fugacity  $f_3 = 5.58 \cdot 10^5 \text{ bar}$  (blue histogram in Fig. S3-a) is especially interesting, since the system is approaching the step in the adsorption isotherm, and the resulting intercell correlations are very strong. Even the IPA approach encounters some difficulty in matching the probability distributions with the same excellent accuracy it granted in other conditions. Nevertheless, the CG-IPA provides an agreement with FG that is far more satisfactory than the CG-NIPA.

## II. LENNARD-JONES SYSTEM

### A. Coarse-graining of a lone pair of pores under the NIPA

We provide adsorption isotherms for the ‘lone-pair-of-pores’ version of the Lennard-Jones system of methane molecules (united atom approximation) under the static field of the zeolite ITQ-29 framework, where the configurations of methane molecules in *only two neighboring pores are sampled*, through standard Metropolis grand-canonical Monte Carlo (GCMC), while the rest of the system is being kept empty. Under such conditions, the *non-interacting pair approximation* (NIPA) applies [see Eq. (21) in the main article]. Adsorption isotherms for the lone pair are reported as empty circles in Fig. S4, at the temperatures of 100, 200, 300, 400, and 500 K. The corresponding adsorption isotherms for the whole system are reported as well (small red dots), in order to highlight the different adsorption properties that emerge as an effect of considering a pair of neighboring pores as it were separated from the rest of the system. We estimated the effective interaction parameters for the coarse-grained (CG) version of the lone pore pair system under the NIPA, and used them to calculate adsorption isotherms (solid blue lines). The agreement is very good, because the NIPA refers precisely to a lone pair of pores. However, once used for CG simulations of the whole system, where pore pairs interact with their surroundings, the NIPA parameters provide a less accurate representation than the ones calculated under the *interacting pair approximation* (IPA) described in the main article.

### B. Coarse-graining of the full LJ systems

We provide the same kind of data we provided in Section I, but here referred to the coarse-graining of the Lennard-Jones system, as a whole.

## III. ESTIMATION OF THE INTERACTION TERMS

We describe two possible routes for the estimation of the interaction terms  $Q_n$  and  $Z_{n_1, n_2}$ .

### A. ‘One-chemical-potential-at-a-time’ (OCT)

In this strategy, first we obtained  $\mu$ -dependent CG interactions, and then we removed the  $\mu$ -dependency through a weighted average.

In the first step, we made use of

$$\frac{Q_n}{Q_{n'}} \approx e^{-\beta\mu(n-n')} \frac{P_\mu^o(n)}{P_\mu^o(n')}. \quad (\text{S3})$$

and of

$$\frac{Z_{n_1, n_2}}{Z_{n'_1, n'_2}} \approx \left( e^{-\beta\mu(n_1+n_2-n'_1-n'_2)} \frac{Q_{n'_1} Q_{n'_2}}{Q_{n_1} Q_{n_2}} \right)^{\frac{1}{\nu}} \left( \frac{P_\mu(n'_1) P_\mu(n'_2)}{P_\mu(n_1) P_\mu(n_2)} \right)^{1-\frac{1}{\nu}} \frac{P_\mu(n_1, n_2)}{P_\mu(n'_1, n'_2)}. \quad (\text{S4})$$

in order to estimate the interaction parameters recursively *for each chemical potential*, with  $n' = n + 1$  in (S3), and with  $n'_1 = n_1 - 1 \wedge n'_2 = n_2$  [contributing with a weight  $\propto P_\mu(n_1 - 1, n_2)$ ] and  $n'_1 = n_1 \wedge n'_2 = n_2 - 1$  [contributing with a weight  $\propto P_\mu(n_1, n_2 - 1)$ ] in (S4). In the second step, the chemical potential-dependence of the parameters  $Q_n(\mu)$  and  $Z_{n_1, n_2}(\mu)$  resulting from the first step was removed by means of weighted averages:  $Q_n = \sum_{\mu \in \{\mu\}} \omega_n(\mu) Q_n(\mu)$  and  $Z_{n_1, n_2} = \sum_{\mu \in \{\mu\}} \omega_{n_1, n_2}(\mu) Z_{n_1, n_2}(\mu)$ , where the weights were set as proportional to the frequency with which each occupancy (or occupancy pair) was sampled in the FG systems of reference:  $\omega_n(\mu) = P_\mu^o(n) / \sum_{\mu' \in \{\mu\}} P_{\mu'}^o(n)$ , and  $\omega_{n_1, n_2}(\mu) = P_\mu(n_1, n_2) / \sum_{\mu' \in \{\mu\}} P_{\mu'}(n_1, n_2)$ .

### B. ‘Choose-the-best-ratio’ (CBR)

In this strategy, first we computed the  $\mu$ -dependent ratios  $R_n^\Delta(\mu)$  [defined as the R.H.S. of Eq. (S3)] and  $R_{n_1, n_2}^{\Delta_1, \Delta_2}(\mu)$  [defined as the R.H.S. of Eq. (S4)], with  $1 \leq \Delta \leq n$ ,  $1 \leq \Delta_1 \leq n_1$ ,  $1 \leq \Delta_2 \leq n_2$ , and  $\Delta_1 \neq \Delta_2$ , and then (ii) we removed the  $\mu$ -dependence by simply selecting, for each doublet  $n, \Delta$  and for each quadruplet,  $n_1, \Delta_1, n_2, \Delta_2$ , the one value,  $R_n^\Delta$ , out of the candidates  $R_n^\Delta(\mu_1), R_n^\Delta(\mu_2), \dots$ , and the one value,  $R_{n_1, n_2}^{\Delta_1, \Delta_2}$ , out of the candidates  $R_{n_1, n_2}^{\Delta_1, \Delta_2}(\mu_1), R_{n_1, n_2}^{\Delta_1, \Delta_2}(\mu_2), \dots$ , that we found to be the most representative ones. Our selection criteria were the magnitude of the probabilities involved (the higher, the better) and the ‘distance’ between the probabilities at the numerator and the ones at the denominator (the more similar the probabilities, the more similar the accuracies). Finally, (iii) we applied the same criteria to select the best  $R_n^{\Delta*}$  out of the set  $\{R_n^\Delta\}_{\Delta=1, \dots, n}$ , and the best  $R_{n_1, n_2}^{\Delta_1^*, \Delta_2^*}$  out of the set  $\{R_{n_1, n_2}^{\Delta_1, \Delta_2}\}_{\Delta_1, \Delta_2}$ , and calculated recursively  $Q_n = R_n^{\Delta*} Q_{n-\Delta*}$ , and  $Z_{n_1, n_2} = R_{n_1, n_2}^{\Delta_1^*, \Delta_2^*} Z_{n_1-\Delta_1^*, n_2-\Delta_2^*}$ .

In general, one cannot expect the OCT and CBR approach to provide *exactly coincident* parameter sets. In the simulations we performed, in some cases, one method provided slightly better results than the other, and in other cases, the difference between one method and the other was very hard to notice. A much more important role than the choice of the OCT or CBR approach was played by the magnitude of the probabilities involved in (S3) and (S4), which were estimated as histograms from GCMC simulations of the FG system. We carried out the calculation of the ratios in (S3) and (S4) only for those values of  $\mu$  for which the probabilities involved were above some threshold, that was set as  $tP_{\max, \mu}^{(1)}$  for (S3) [where  $P_{\max, \mu}^{(1)}$  is the maximum probability value observed in the histogram  $P_\mu(\cdot)$ ], and  $tP_{\max, \mu}^{(2)}$  for (S4) [where  $P_{\max, \mu}^{(2)}$  is the maximum probability value observed in the bivariate histogram  $P_\mu(\cdot, \cdot)$ ]. For each FG system, the threshold  $t$  was treated as an adjustable parameter with optimal values in the range  $10^{-5} < t < 10^{-3}$ .

Properly adjusting  $t$  led to significantly reducing the noise in the CG simulations produced by the inaccuracy that unavoidably affects the estimation of probabilities of infrequent events. Moreover, one should notice that the approximation (S4) is, in general, weaker than the approximation (S3). The reason is that, while approximation (S3) relies on Eq. (13) of the main article, which is exact [so that the histogram  $P_\mu^o(\cdot)$ , as evaluated from GCMC, suffers only from the finite simulation length], approximation (S4) instead relies on Eq. (15) of the main article, which in turn *relies on the approximation*  $P_\mu(n_1, n_2) \approx p_\mu(n_1, n_2)$ , rather than on some equality. That represents an additional source of noise in the evaluation of the pair terms  $Z_{n_1, n_2}$ , and makes the role of the threshold  $t$  even more important in the evaluation of CG pair interactions.

### C. Missing entries in the CG interaction matrix

As we mentioned in the main article, depending on the features of the systems under study, it is possible that some neighboring occupancy pairs are never sampled at any of the chemical potentials at which the GCMC simulations are performed, causing some entries in the interaction matrix  $K_{n_1, n_2}$  (or, equivalently,  $Z_{n_1, n_2}$ ) to be missing [see Eq. (S4)]. However, this does not really constitute a problem, since the CG system will simply not sample the occupancy pairs that neither were not sampled in the original FG system. [?] The only thing that matters is that enough interaction terms could be evaluated, so that the CG system can correctly sample the same occupancy configurations that were sampled in the original system, saturating correctly, rather than, e.g., remaining stuck at some intermediate density because of the lack of pair terms at high occupancies. This depends on how accurately the occupancy distributions in the FG system are determined. In earlier works, the NIPA approach was used along with expanded ensemble methods (EEM), [?] which in this case would essentially prescribe, during the simulation of the pair as separated from the rest of the system, to assign each pore a different (fictitious) chemical potential, and to find conditions allowing the sampling of all possible pair occupancies, including those that would actually never be sampled by the original FG system, in which the chemical potential is homogeneous. In all the cases we investigated, we found that the NIPA pair-interaction terms, calculated by recursively solving for  $Z_{n_1, n_2}^*$  in Eq. (21) in the main article (with the same procedure we adopted in our previous work about this subject [?]), gave a perfect agreement between isotherms and occupancy distributions of the NIPA system itself (see Supplementary Material), thus basically confirming that, for our purpose of producing the CG version of some FG system at thermodynamic equilibrium, the lack of sampling of pair occupancies that are never sampled in the original system does not affect the quality of the agreement between CG and FG occupancy distributions.

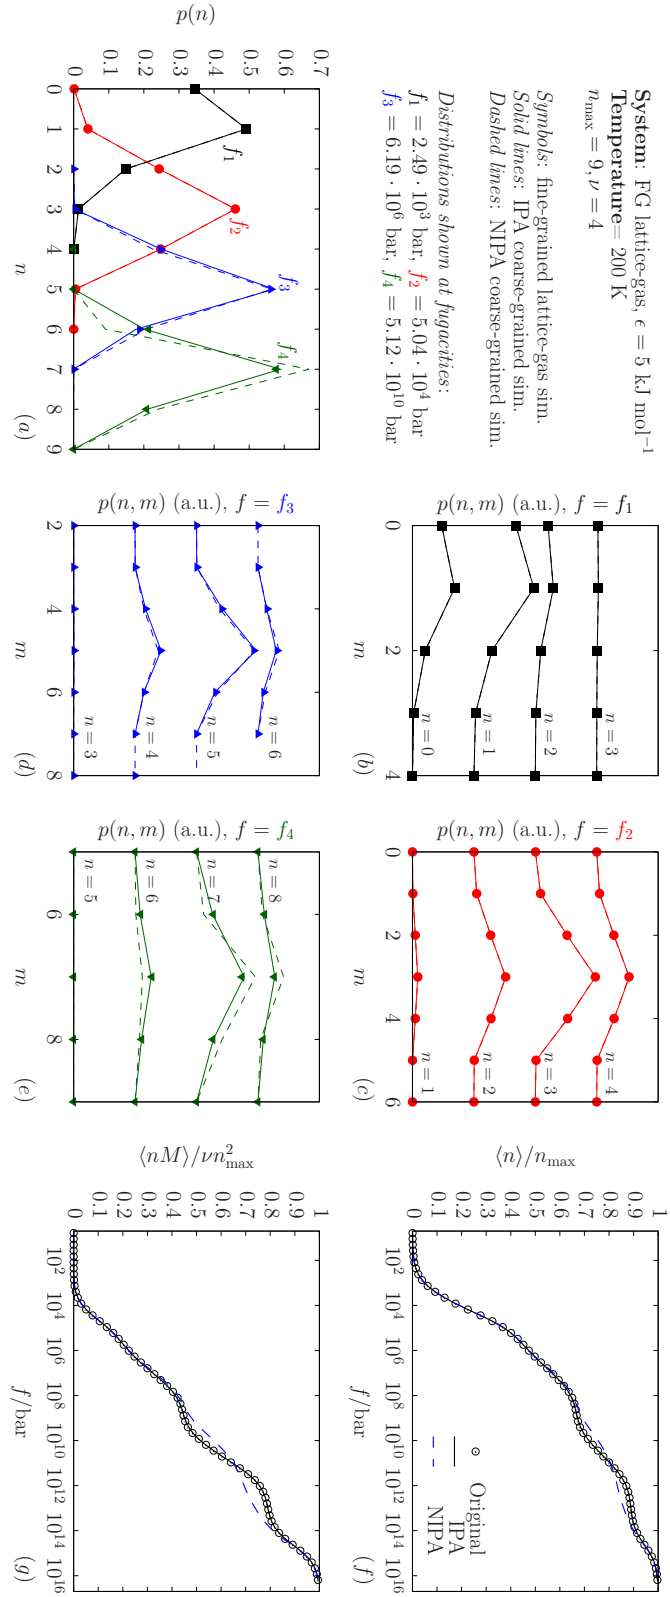

FIG. S1: Selected (a) single-pore and (b-e) pore-pair occupancy distributions, along with (f) the adsorption isotherm and (g) a plot of the extended density *vs.* the fugacity, for a version of the lattice-gas system in which only plain lateral repulsions are present, and are set to the value of  $5 \text{ kJ mol}^{-1}$ .

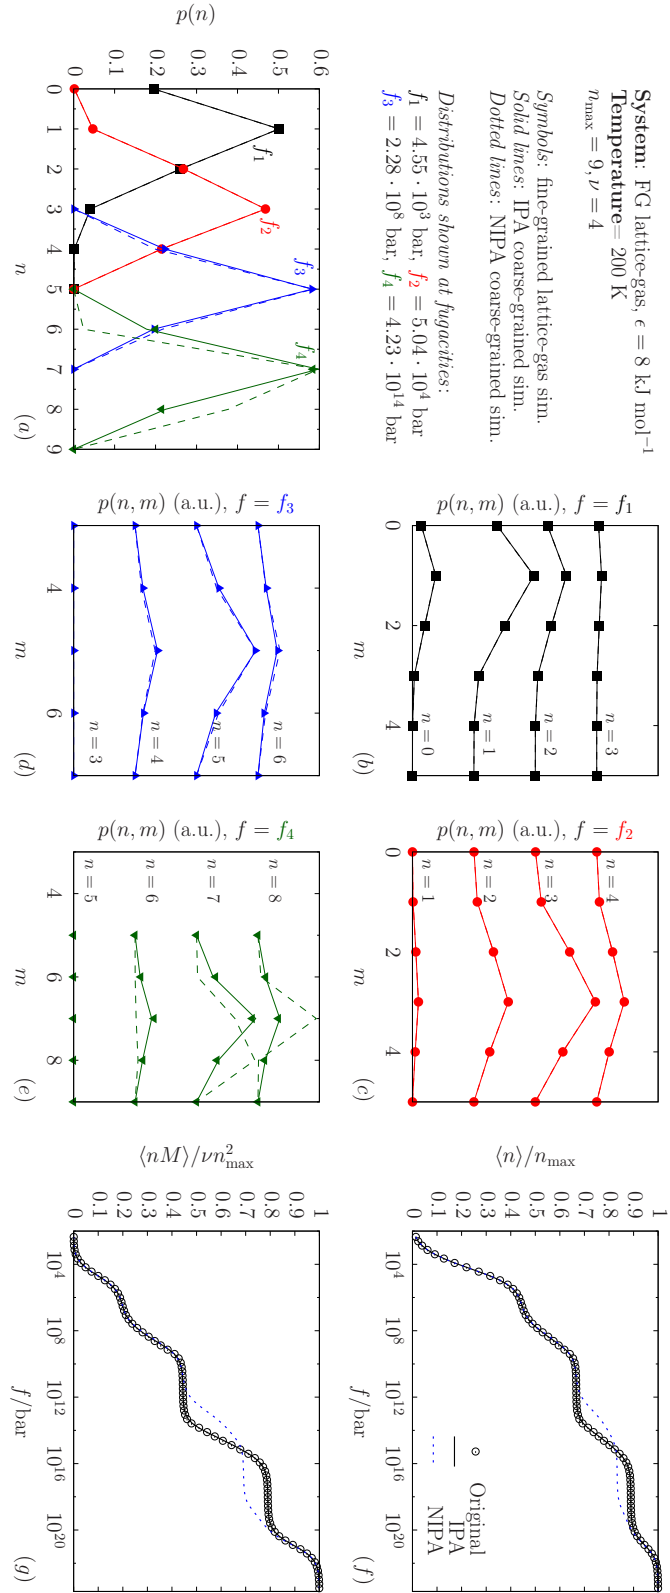

FIG. S2: Selected (a) single-pore and (b-e) pore-pair occupancy distributions, along with (f) the adsorption isotherm and (g) a plot of the extended density *vs.* the fugacity, for a version of the lattice-gas system in which only plain lateral repulsions are present, and are set to the value of  $8 \text{ kJ mol}^{-1}$ .

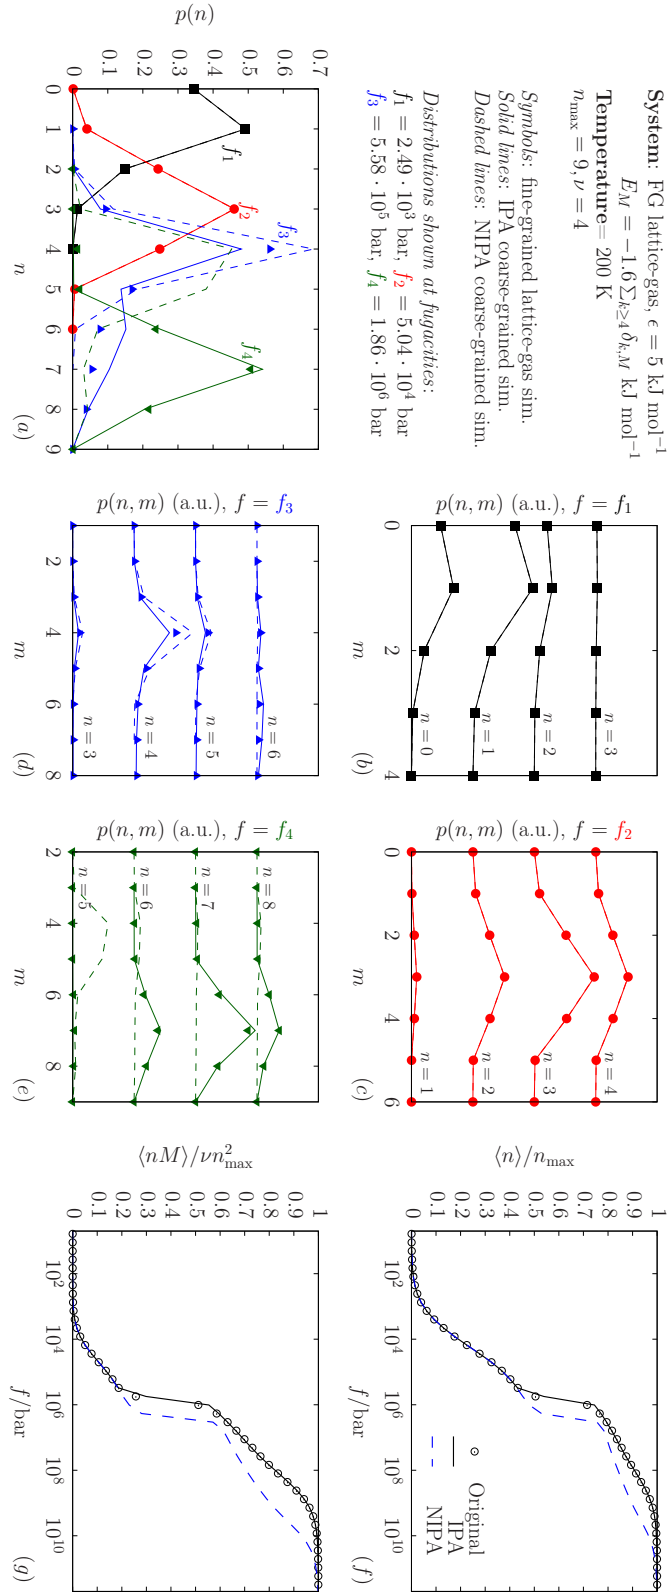

FIG. S3: Selected (a) single-pore and (b-e) pore-pair occupancy distributions, along with (f) the adsorption isotherm and (g) a plot of the extended density *vs.* the fugacity, for a version of the lattice-gas system in which lateral repulsions are set to the value of  $5 \text{ kJ mol}^{-1}$ , and extended interactions are added according to parameter values  $\phi = -1.6 \text{ kJ mol}^{-1}$  and  $M_0 = 4$ .

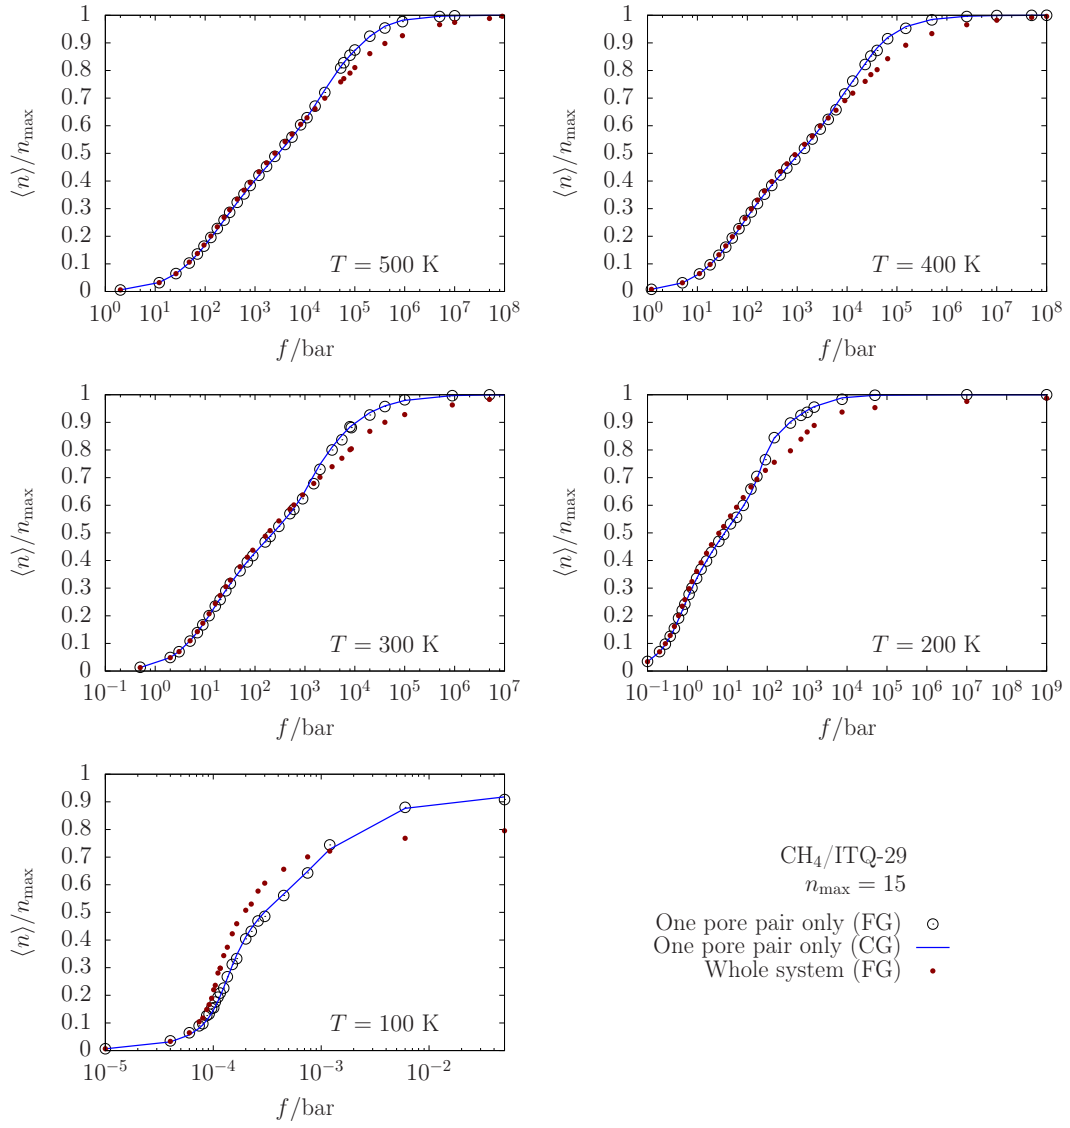

FIG. S4: Adsorption isotherms at various temperatures for a version of the Lennard-Jones system we considered in the main article, in which the adsorption of methane molecules inside of only two neighboring ITQ-29 pores is simulated through GCMC. Data from fine-grained simulations (empty circles) are shown together with data from the coarse-grained version of the same system (solid blue lines), in which we used the effective interaction parameters calculated under the NIPA. Adsorption isotherms for the full (fine-grained) system are reported as well (small red dots).

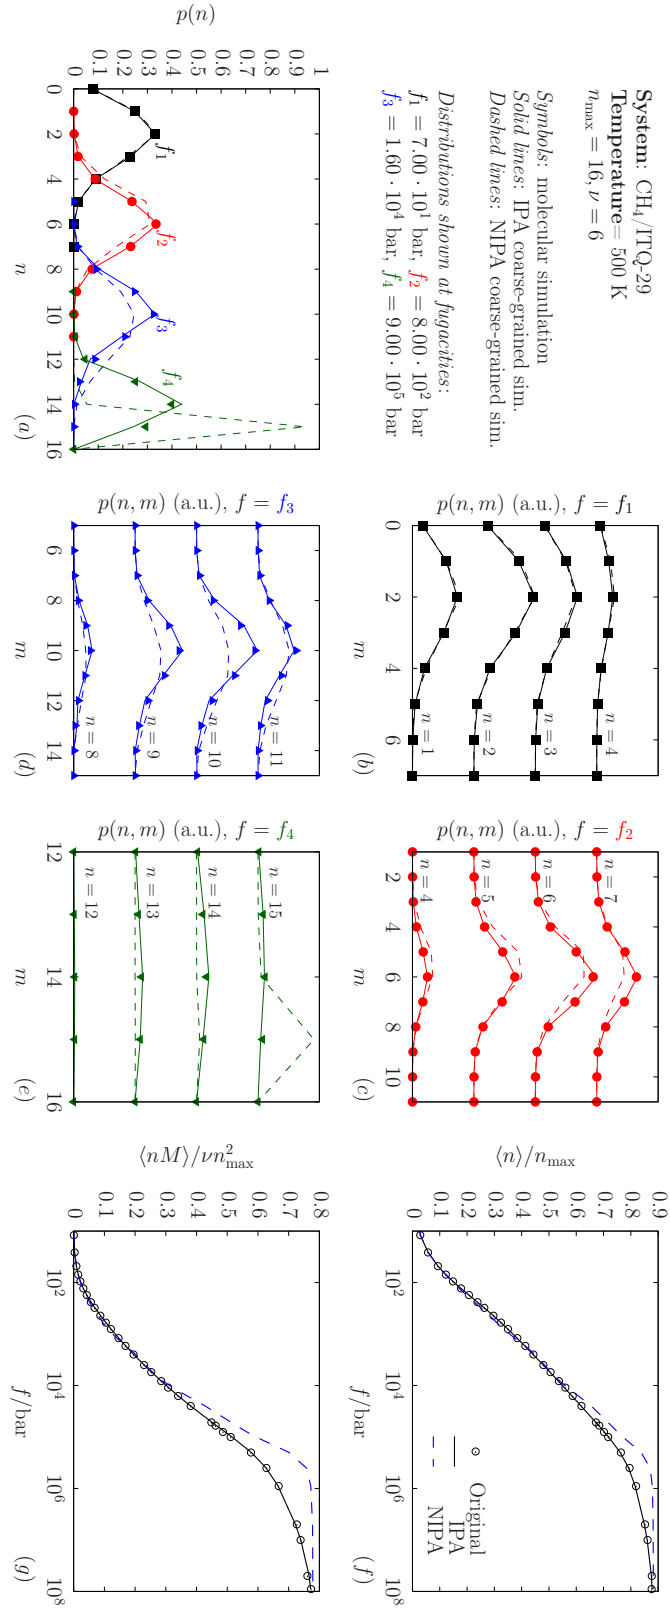

FIG. S5: Selected (a) single-pore and (b-e) pore-pair occupancy distributions, along with (f) the adsorption isotherm and (g) a plot of the extended density *vs.* the fugacity, for the Lennard-Jones (united-atom-CH<sub>4</sub>)/(static-ITQ-29) system at the temperature of 500 K.

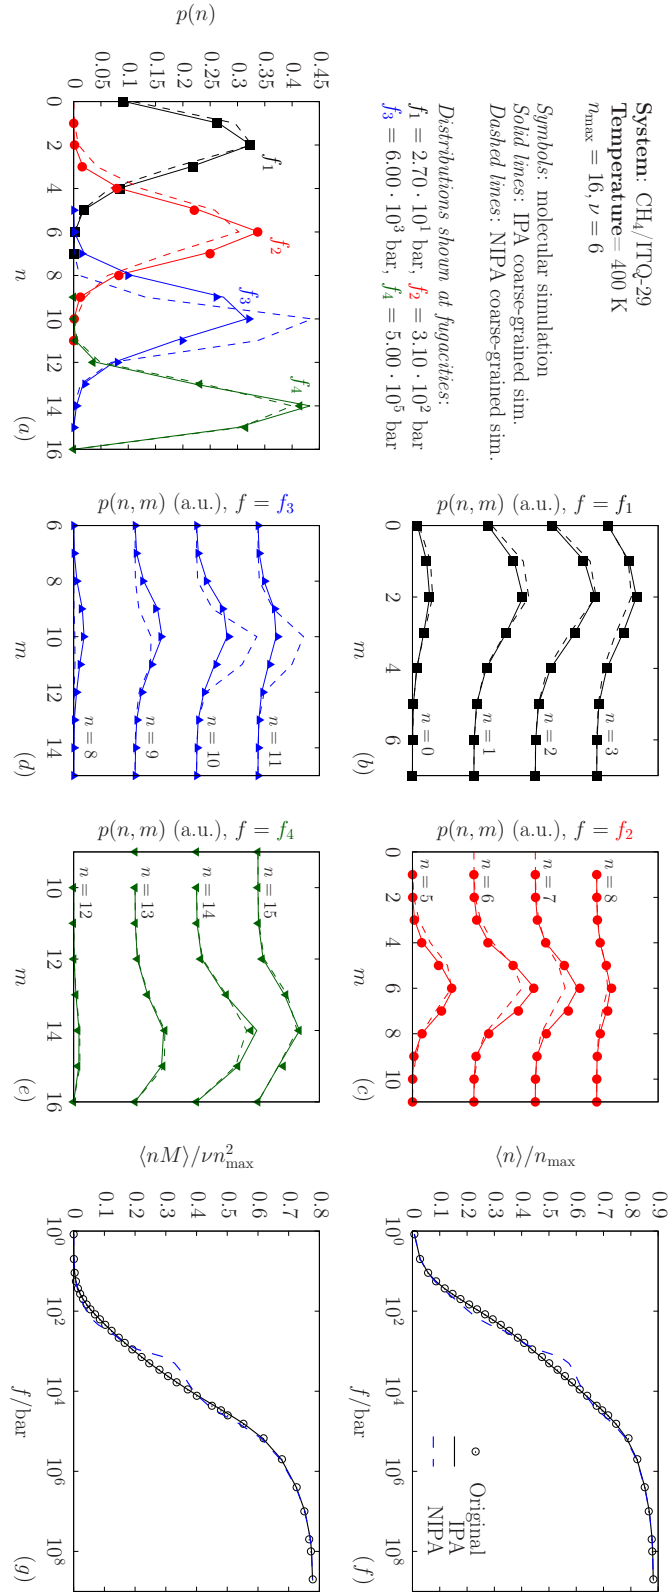

FIG. S6: Selected (a) single-pore and (b-e) pore-pair occupancy distributions, along with (f) the adsorption isotherm and (g) a plot of the extended density *vs.* the fugacity, for the Lennard-Jones (united-atom-CH<sub>4</sub>)/(static-ITQ-29) system at the temperature of 400 K.

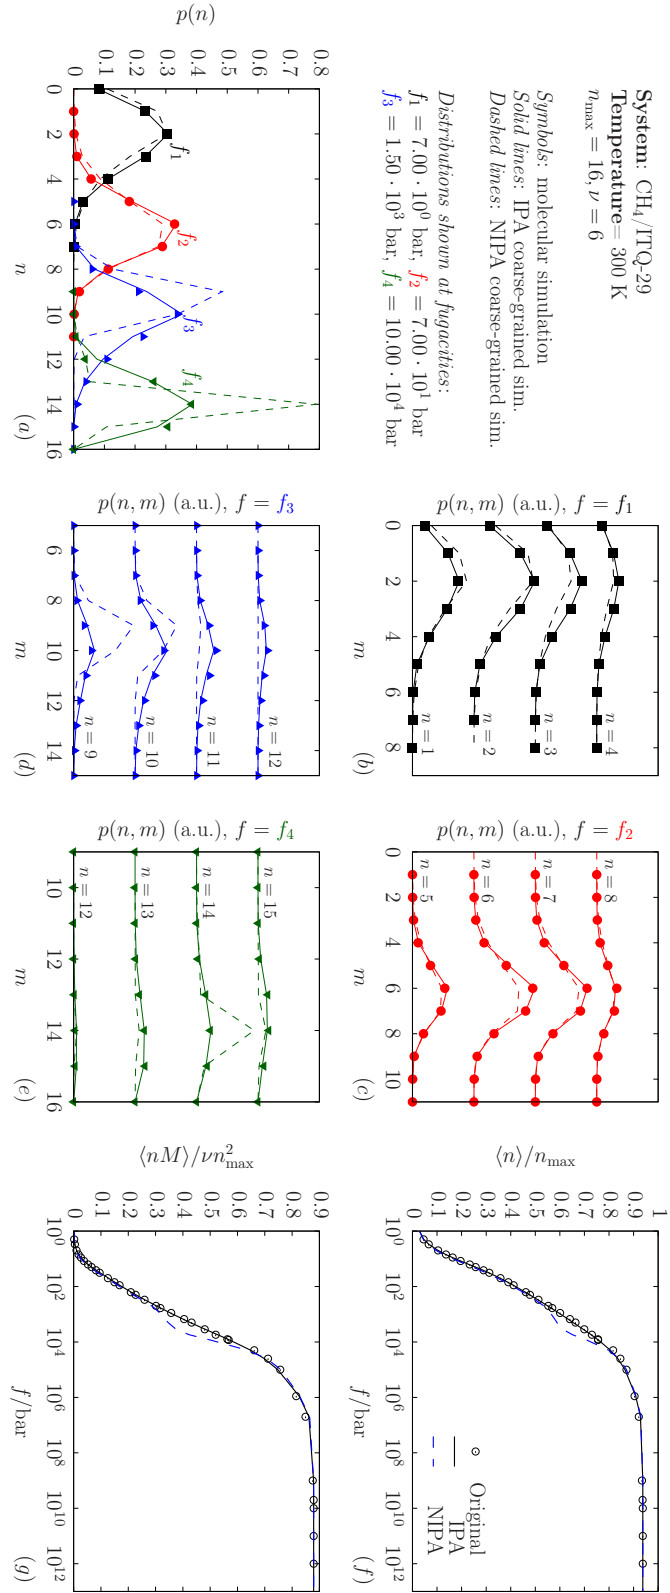

FIG. S7: Selected (a) single-pore and (b-e) pore-pair occupancy distributions, along with (f) the adsorption isotherm and (g) a plot of the extended density *vs.* the fugacity, for the Lennard-Jones (united-atom-CH<sub>4</sub>)/(static-ITQ-29) system at the temperature of 300 K.

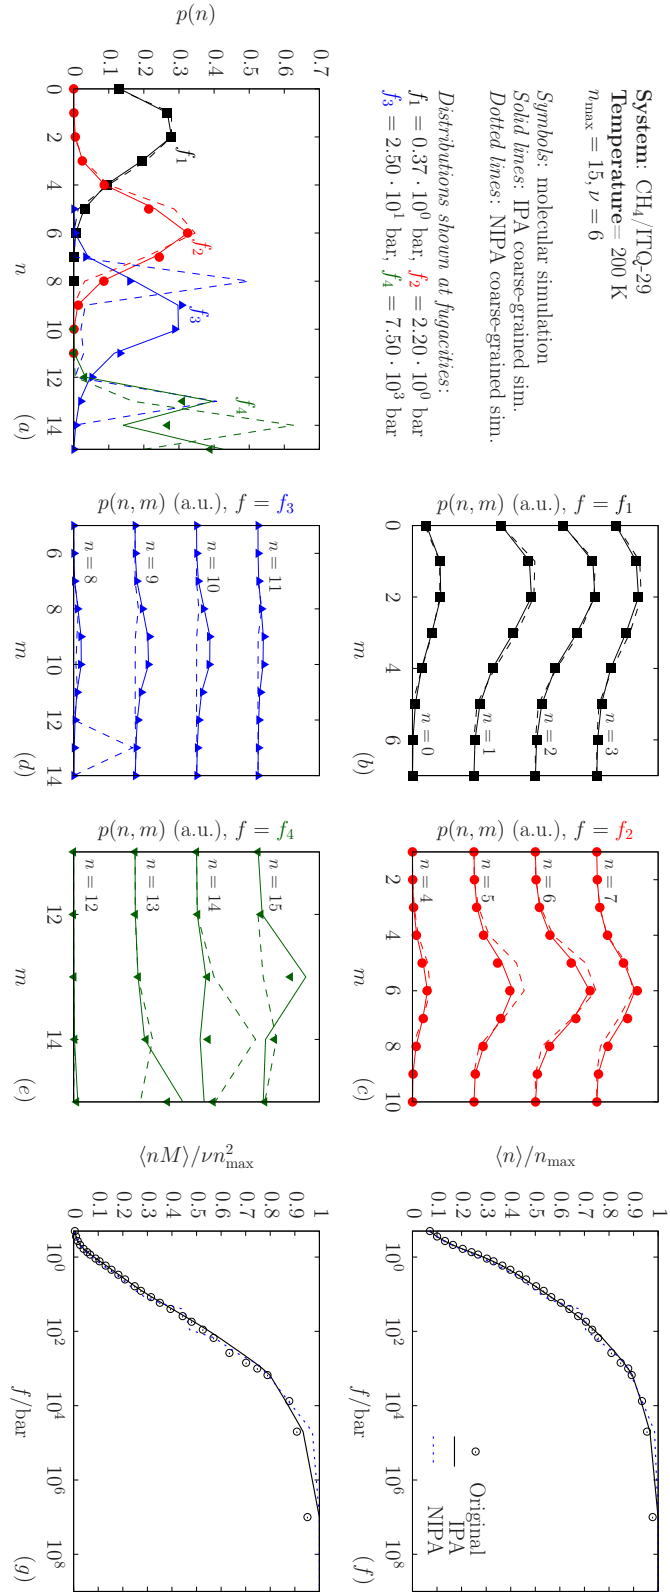

FIG. S8: Selected (a) single-pore and (b-e) pore-pair occupancy distributions, along with (f) the adsorption isotherm and (g) a plot of the extended density *vs.* the fugacity, for the Lennard-Jones (united-atom-CH<sub>4</sub>)/(static-ITQ-29) system at the temperature of 200 K.

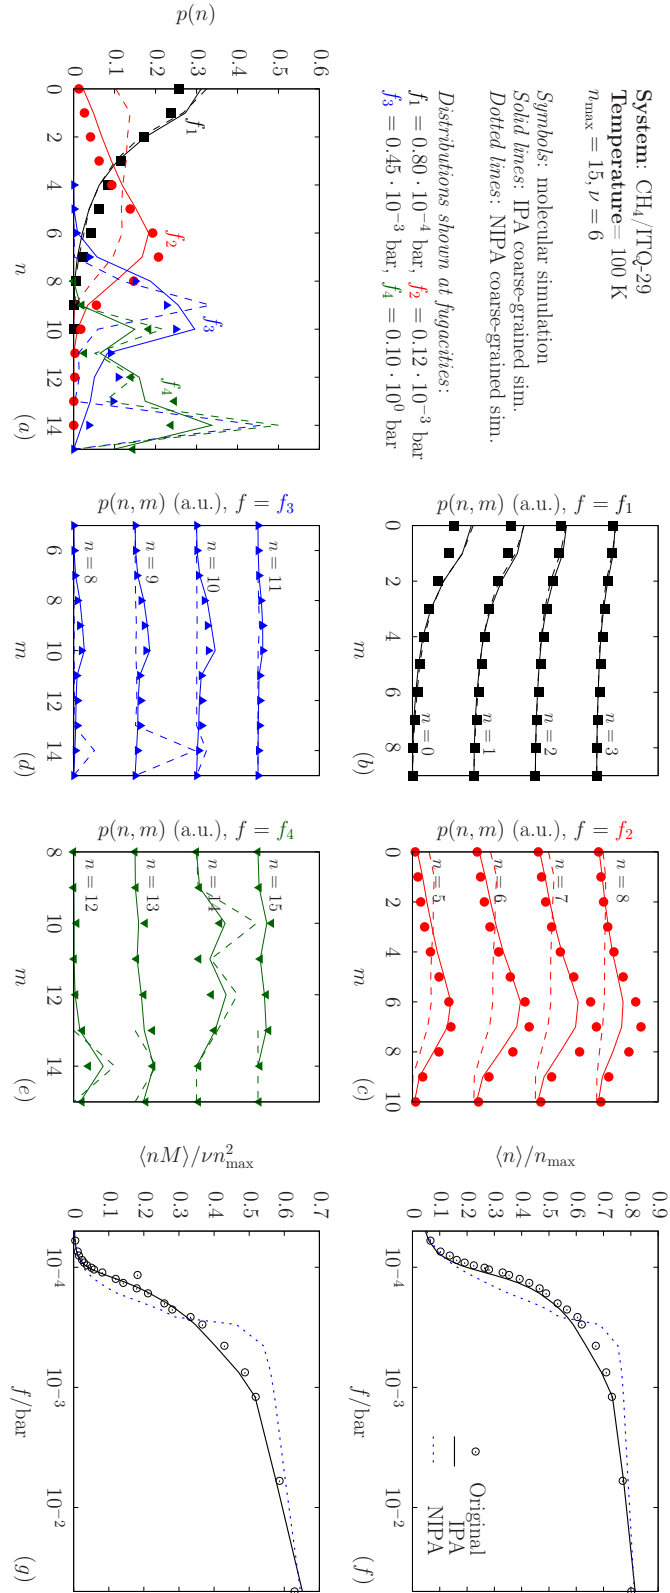

FIG. S9: Selected (a) single-pore and (b-e) pore-pair occupancy distributions, along with (f) the adsorption isotherm and (g) a plot of the extended density *vs.* the fugacity, for the Lennard-Jones (united-atom-CH<sub>4</sub>)/(static-ITQ-29) system at the temperature of 100 K.
